# Supplementary material for: Cooperative-Memory Photonic Reservoir using Modulation Nonlinearity: Circumventing the Speed Constraints of Nonlinear Silicon Microring Resonators
Source: arXiv:2504.16422 source file (2025-04-23)
Supplement: Supplementary file 1 [file Supplementary.pdf]

# Cooperative-Memory Photonic Reservoir using Modulation Nonlinearity: Circumventing the Speed Constraints of Nonlinear Silicon Microring Resonators

Amideddin Mataji-Kojouri[1]*, Sebastian Kühl[2],

Mohammad Seifi Laleh[2], Stephan Pachnicke[2], Kambiz Jamshidi[1]*

[1]*Integrated Photonic Devices Group, Chair of RF and Photonics Engineering, TU Dresden, Helmholzstr. 18, Dresden, 01069, Germany.

[2]Chair of Communications, Kiel University, Kaiserstr. 2, Kiel, 24143, Germany.

*Corresponding author(s). E-mail(s): amideddin.matajikojouri@tu-dresden.de; kambiz.jamshidi@tu-dresden.de;

Contributing authors: sk@tf.uni-kiel.de; mola@tf.uni-kiel.de; stephan.pachnicke@tf.uni-kiel.de;

## Supplementary Information

Table S1. Parameters of the nonlinear model

| Parameter | Value | Unit |
|---|---|---|
| $n_0$ | 4.1 | - |
| $\alpha_{ring}$ | $46\ (L = 2\ dB/cm)$ | $1/\mathrm{m}$ |
| $\eta_{lin}$ | 0.4 | - |
| $R$ | 10 | μm |
| $n_2$ | $4.5 \times 10^{-18}$ | $\mathrm{m}^2/\mathrm{W}$ |
| $\beta_2$ | $7.5 \times 10^{-12}$ | $\mathrm{m}/\mathrm{W}$ |
| $\sigma_{FCA}$ | $1.45 \times 10^{-21}$ | $\mathrm{m}^2$ |
| $A_{eff}$ | $2.04 \times 10^{-13}$ | $\mathrm{m}^2$ |
| $A_{TPA}$ | $1.289 \times 10^{-13}$ | $\mathrm{m}^2$ |
| $A_{FCA}$ | $1.16 \times 10^{-13}$ | $\mathrm{m}^2$ |
| $\rho_{Si}$ | $2.329 \times 10^{3}$ | $\mathrm{kg}/\mathrm{m}^3$ |
| $c_{Si}$ | 713 | J/(kg K) |
| $k_\theta$ | $1.86 \times 10^{-4}$ | $\mathrm{K}^{-1}$ |

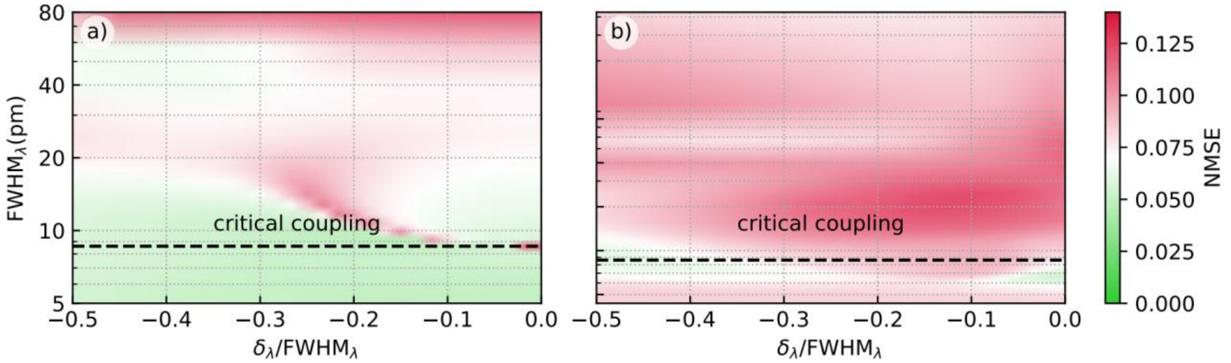


Fig. S1 NMSE for Santa-Fe prediction task, when input is amplitude modulated (a) or phase modulated (b), for different values of normalized detuning and resonator linewidth controlled by the coupling strength.

Table S2. Parameters of the optimized PIC for optical signal equalization

| Parameter | Value | Unit |
|---|---|---|
| MZI delay difference | 4.46 | $ps$ |
| $Q/Q_{int}$ | 0.69 | - |
| MZI input coupling | 0.47 | - |
| MZI output coupling | 0.116 | - |
| Normalized detuning | 0.843 | - |
